# Supplementary material for: Temperature-dependent templated growth of porphine thin films on the (111) facets of copper and silver
Source: arXiv:1407.0486 source file (2014-07-02)
Supplement: Supplementary file 1 [file Diller_TUM_SI.pdf]

# Temperature-dependent templated growth of porphine thin films on the (111) facets of copper and silver

## Supporting Information

Katharina Diller, Florian Klappenberger, Francesco Allegretti, Anthoula C. Papageorgiou, Sybille Fischer, David A. Duncan, Reinhard J. Maurer, Julian A. Lloyd, Seung Cheol Oh, Karsten Reuter, and Johannes V. Barth

## I. X-RAY SPECTROSCOPY DATA: NITROGEN REGION

The XPS and NEXAFS spectra of 2H-P multilayers in the nitrogen region were recorded with the same setup as the corresponding carbon data presented in the manuscript. In order to detect photoelectrons with the same kinetic energy in both C and N regions the photon energy was set to 550 eV, and the retarding voltage for the partial electron yield NEXAFS measurements was set to -250 V. Simulations were carried out according to the procedure described in the manuscript.

As discussed in the manuscript the 2H-P XPS N1s region (Fig. S1) is typical for free-base porphyrins. Our calculation confirms the already well known peak assignment: peak A originates from iminic (N) nitrogen, peak B from pyrrolic (NH) nitrogen. Accordingly, the NEXAFS N K-edge region for porphyrins has five characteristic peaks in the $\pi^*$ region (Fig. S2), resulting from the sum of the two similar nitrogen NEXAFS curves shifted by the characteristic 1s core level energy separation of approximately 2 eV. Tables I, III and II list energy positions and assignment of the experimental and simulated peaks.

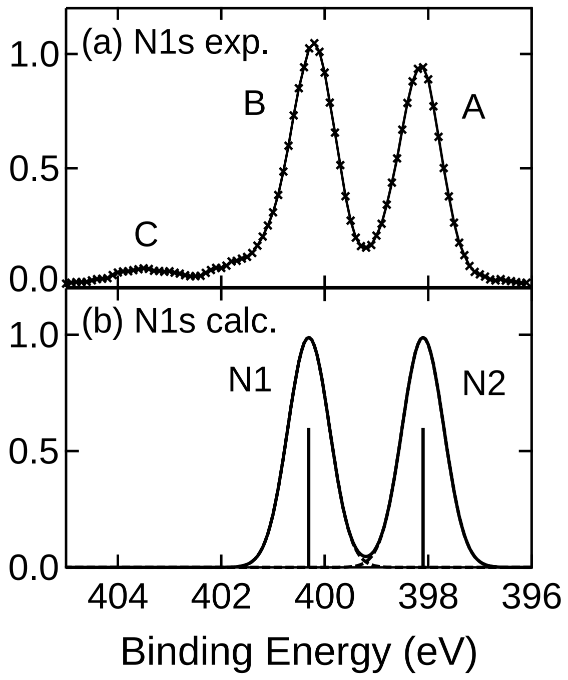


FIG. S**1** N1s XPS signature of porphine. The (a) experimental multilayer curve (2H-P/Cu(111) grown at LT) is very well reproduced by (b) the simulated spectrum. N1: pyrrolic nitrogen (NH), N2: iminic nitrogen (N); peak C at higher binding energies can be assigned to a shake up peak and therefore does not appear in the simulated spectrum.

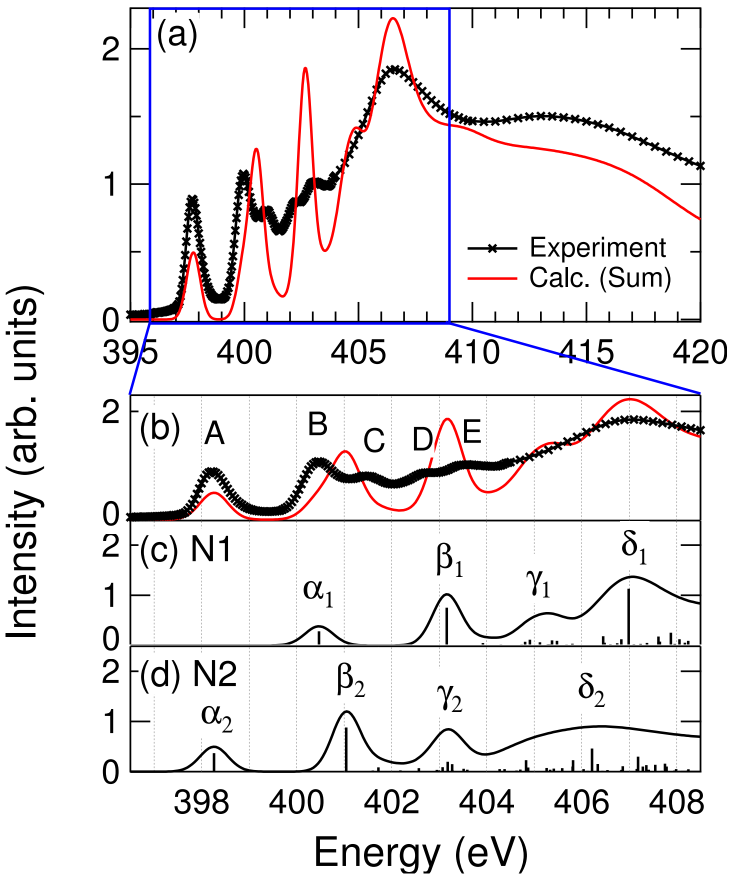


FIG. S**2** NEXAFS N K-edge signature of 2H-P. Panel (a) compares the experimental curve at the "magic angle" (53°) for a 2H-P multilayer (black markers) with the simulated spectrum (red continuous line). The (b) zoom-in and (c-d) the curves originating from the two inequivalent nitrogen atoms show that the spectrum can be deconvoluted in the two contributions originating from the iminic (N) and the pyrrolic (NH) nitrogen species.

TABLE I: Calculated ionization energies ($E_{calc}$) for the inequivalent N and C species. $E_{calc}$ (shifted) displays the same energies after shifting them by -4.45 eV (C) and -4.21 eV (N) for a better comparison with the experimental data. The energy shift, Δ, is referenced against N2 or C5 (cf. Fig. 1a).

| Atom | $E_{calc}$ | $E_{calc}$ (shifted) | Type | Δ | Peak |
|---|---|---|---|---|---|
| N1 | 404.5 eV | 400.3 eV | -NH- | 2.2 eV | B |
| N2 | 402.3 eV | 398.1 eV | =N- | 0.0 eV | A |
| | | | | | |
| C1 | 289.2 eV | 284.8 eV | C-C | 0.3 eV | D |
| C2 | 290.2 eV | 285.8 eV | C-NH | 1.3 eV | E |
| C3 | 289.0 eV | 284.6 eV | C-C | 0.1 eV | D |
| C4 | 289.7 eV | 285.2 eV | C-N | 0.8 eV | E |
| C5 | 288.9 eV | 284.4 eV | C-C | 0.0 eV | D |

TABLE II: Peak assignment for the 2H-P N K-edge NEXAFS spectrum

| Peak[a] | Peak[b] | Exp.[c] | Comp.[d] | Type[e] | Transition[f] |
|---|---|---|---|---|---|
| A | $\alpha_2$ | 397.7 eV | 397.8 eV | =N- | 1. (1s) $\rightarrow$ 79. (LUMO) |
| B | $\alpha_1$ | 400.0 eV | 400.0 eV | -NH- | 1. (1s) $\rightarrow$ 79. (LUMO) |
| C | $\beta_2$ | 401.0 eV | 400.5 eV | =N- | 1. (1s) $\rightarrow$ 82. (LUMO+3) |
| D-E | $\beta_1$ | 402.1-403.1 eV | 402.7 eV | -NH- | 1. (1s) $\rightarrow$ 82. (LUMO+3) |
| | $\gamma_2$ | | 402.7 eV | =N- | several |

[a] Peaks in experimental spectra
[b] Peaks in computed spectra
[c] Experimental peak positions
[d] Computed peak positions (shifted by 0.1 eV to match experimental spectrum)
[e] Atom type of excitation center: $n = 0.5$ in TP calculation
[f] Transition (orbital numbers)

TABLE III: Peak assignment for the 2H-P C K-edge NEXAFS spectrum

| Peak[a] | Peak[b] | Exp.[c] | Comp.[d] | Type[e] | Transition[f] |
|---|---|---|---|---|---|
| A | $\alpha_5$ | 284.2 eV | 284.2 eV | C-C | 5. (1s) $\rightarrow$ 63. (LUMO) |
| | $\alpha_3$ | | 284.2 eV | C-C | 5. (1s) $\rightarrow$ 63. (LUMO) |
| | $\alpha_1$ | | 284.5 eV | C-C | 5. (1s) $\rightarrow$ 63. (LUMO) |
| B | $\delta_4$ | 285.0 eV | 285.0 eV | C-N | 5. (1s) $\rightarrow$ 63. (LUMO) |
| | $\delta_2$ | | 285.5 eV | C-NH | 5. (1s) $\rightarrow$ 63. (LUMO) |
| C | $\beta_5$ | 285.7 eV | 285.6 eV | C-C | 5. (1s) $\rightarrow$ 65. (LUMO+2) |
| | $\beta_3$ | | 285.7 eV | C-C | 5. (1s) $\rightarrow$ 65. (LUMO+2) |
| | $\beta_1$ | | 285.9 eV | C-C | 5. (1s) $\rightarrow$ 65. (LUMO+2) |
| D | $\gamma_5$ | 287.4 eV | 287.2 eV | C-C | 5. (1s) $\rightarrow$ 67. (LUMO+4) |
| | $\gamma_3$ | | 287.2 eV | C-C | 5. (1s) $\rightarrow$ 66. (LUMO+3) |
| | $\gamma_1$ | | 287.5 eV | C-C | 5. (1s) $\rightarrow$ 67. (LUMO+4) |
| | $\epsilon_4$ | | 287.8 eV | C-N | 5. (1s) $\rightarrow$ 66. (LUMO+3) |
| E | $\epsilon_2$ | 288.3 eV | 288.2 eV | C-NH | 5. (1s) $\rightarrow$ 66. (LUMO+3) |

[a] Peaks in experimental spectra
[b] Peaks in computed spectra
[c] Experimental peak positions
[d] Computed peak positions (shifted by 0.1 eV to match experimental spectrum)
[e] Atom type of excitation center: $n = 0.5$ in TP calculation
[f] Transition (orbital numbers)

## II. PORPHINE MULTIMERS AND CHAINS

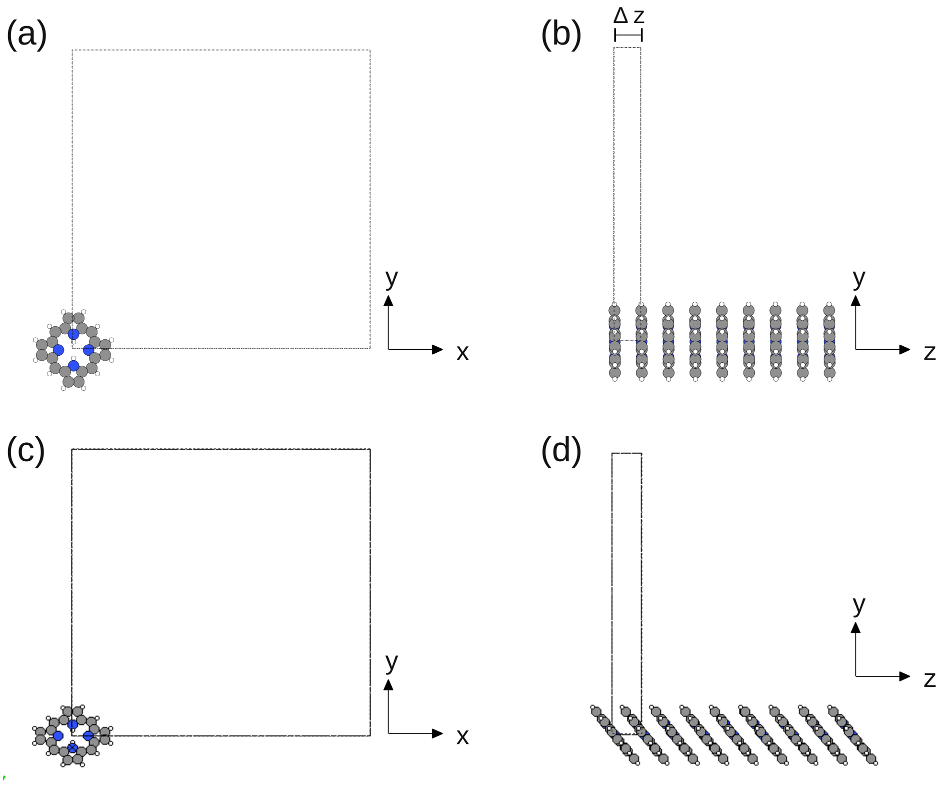


FIG. S**3** Unit cell for stacking of 2H-P along the z-axis. (a) top and (b) side view of symmetric porphine chain; (c) top and (d) side view of tilted porphine chain.

TABLE IV: Details of the optimized dimer geometries shown in Fig. 2. The atom coordinate averages for each molecule were calculated assuming that the deformation of the porphines is small. $d$ and $a$ are defined as the distances between the averaged centers. $a_x$ ($a_y$) is the displacement of this center of mass in x (y), and $a$ is given by $a = \sqrt{a_x^2 + a_y^2}$. For comparison the distances were determined both for all atoms and only for taking into account the nitrogen atoms. $\beta$ describes how the two molecules are rotated with respect to each other. The values are in good agreement with those reported in ref. 1.

| | | all atoms | | | | only N | | | |
|---|---|---|---|---|---|---|---|---|---|
| | $\beta$ | $d$ [Å] | $a_x$ [Å] | $a_y$ [Å] | $a$ [Å] | $d$ [Å] | $a_x$ [Å] | $a_y$ [Å] | $a$ [Å] |
| Dimer 1 | 0 | 3.66 | 0.06 | 0.06 | 0.08 | 3.63 | 0.00 | 0.00 | 0.00 |
| Dimer 2 | 90° | 3.63 | 0.00 | 0.00 | 0.00 | 3.58 | 0.00 | 0.00 | 0.00 |
| Dimer 3 | 0 | 3.43 | 1.14 | 1.05 | 1.55 | 3.42 | 1.07 | 1.07 | 1.51 |
| Dimer 4 | 90° | 3.34 | 1.16 | 1.20 | 1.67 | 3.34 | 1.16 | 1.17 | 1.65 |

TABLE V: Molecular binding energies $E_b$ and molecule-molecule distances $d$: symmetric stacking (cf. Fig. S3 and Fig. 2), geometries optimized with tier 2 basis sets using dispersion corrections, energies determined with tier 2 basis sets.

| | Dimer | Trimer | Tetramer | Pentamer | Periodic |
|---|---|---|---|---|---|
| $E_b$ [a] | 342 meV | 464 meV | 525 meV | 562 meV | 683 meV |
| $d$ [b] | 3.63 Å | 3.65 Å | 3.63 Å | 3.63 Å | 3.64 Å |

[a] per molecule (for $n$ molecules): $E_{ad} = (n \cdot E_{tot}^{mono} - E_{tot}^{n-mer})/\text{n}$
[b] Periodic: size of unit cell; Rest: like in Table IV, only nitrogen atoms taken into account

TABLE VI: Molecular binding energies $E_b$ using tier 3 basis sets for the four dimers depicted in Fig. 2 and the symmetric and tilted infinite chains determined with periodic boundary conditions (Fig. S3). In all cases the binding energies without semi-empirical van-der-Waals correction $E_b^{PBE}$ are negativ, i.e., the structures are not stable. If dispersion interactions are taken into account, all analysed configurations are stable ($E_b^{vdW} > 0$). In all cases the symmetric (non-displaced) structures are energetically less favourable than the corresponding non-symmetric (displaced) structures.

| | aligned (a = 0) | | | displaced (a ≠ 0) | | |
|---|---|---|---|---|---|---|
| | Dimer 1 | Dimer 2 | Chain | Dimer 3 | Dimer 4 | Chain |
| $E_b^{PBE}$ [a] | -163 meV | -160 meV | - | -134 meV | -130 meV | - |
| $E_b^{vdW}$ [b] | 339 meV | 360 meV | 695 meV | 470 meV | 475 meV | 982 meV |

[a] per molecule without van-der-Waals correction
[b] per molecule including semi-empirical dispersion correction

## III. NEXAFS FITTING

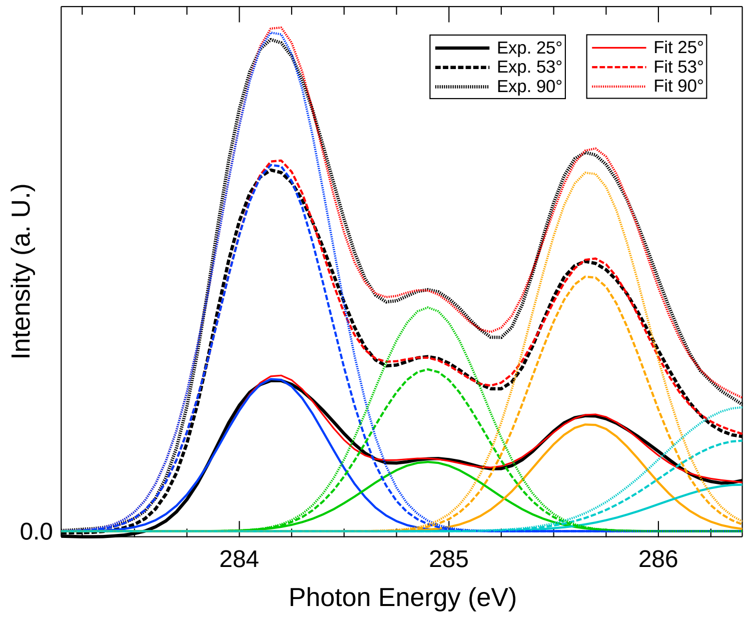


FIG. S**4** Fitting of the experimental NEXAFS curves of a 2H-P multilayer grown at RT on Ag(111) (black): The total curve is approximated by three Gaussians (blue, green, orange). The relative peak intensities of the three Gaussians are then compared to theoretical curves in Figs. 4 and 5.

## IV. SHIFT IN BINDING ENERGIES

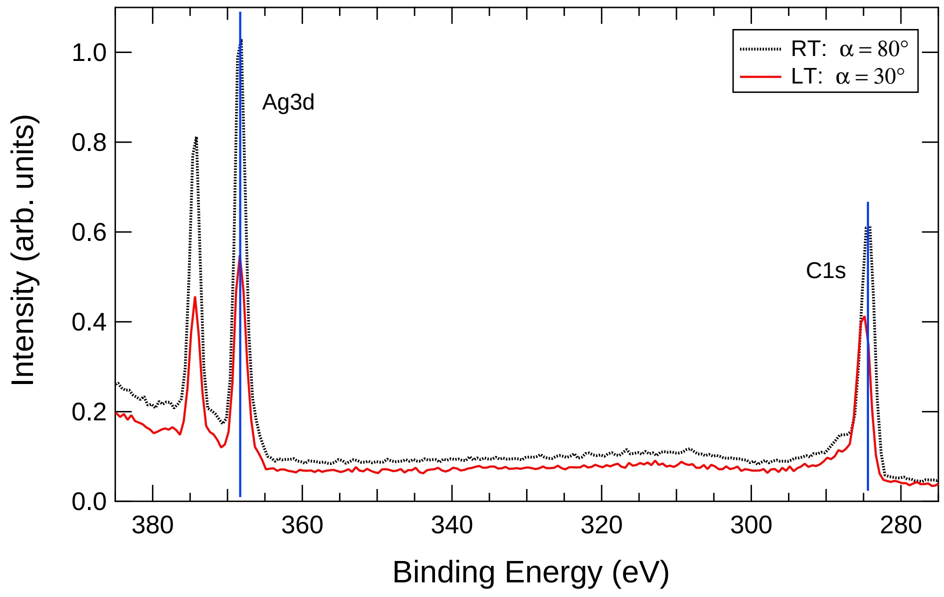


FIG. S**5** Wide area scan XP spectra of 2H-P multilayers grown on Ag(111) at RT and LT

## V. INFLUENCE OF CHLORINE AND OXYGEN MODIFICATIONS ON THE TILTING

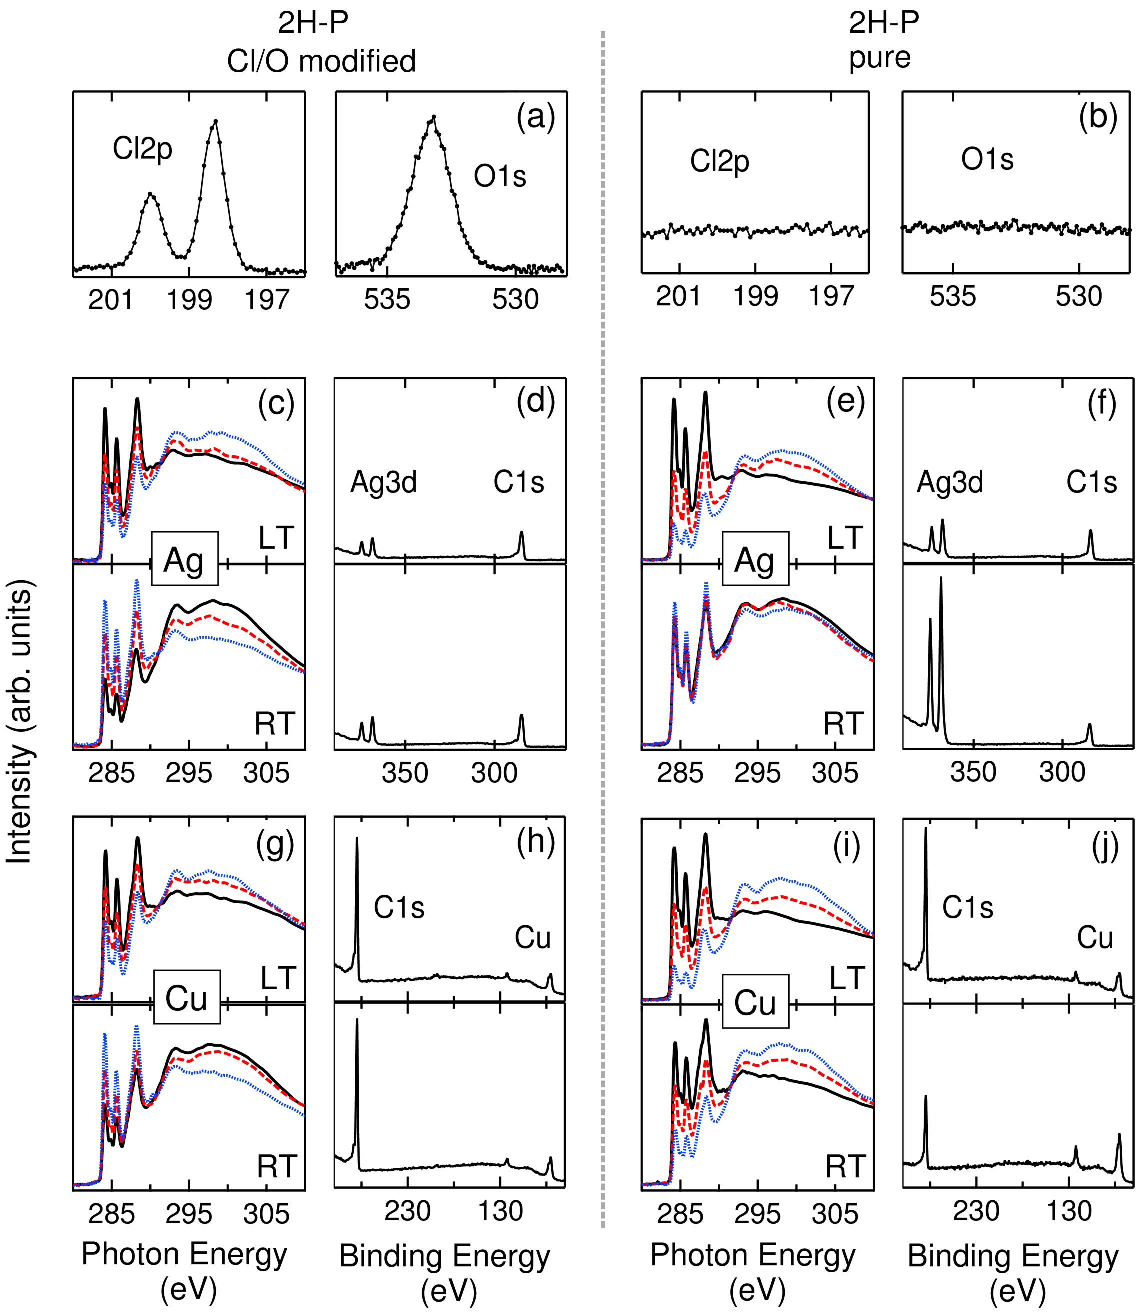


FIG. S**6** Stability and temperature induced re-orientation of 2H-P multilayers on Ag(111) and Cu(111) studied with XPS (d/f, h/j) and angle-resolved NEXAFS (c/e, g/i). The layers of pure porphine adsorbates (right panels) start to re-orient when warming up the sample from low-temperature to room temperature, but also partially desorb as indicated by XPS. Films of 2H-P which were contaminated with Cl are not only stable, but also switch completely from the low-temperature 30° phase to the standing-up phase. Thus, we can obtain perpendicular, $\pi$-stacked layers on both substrates. Cooling down does not change back the orientation.

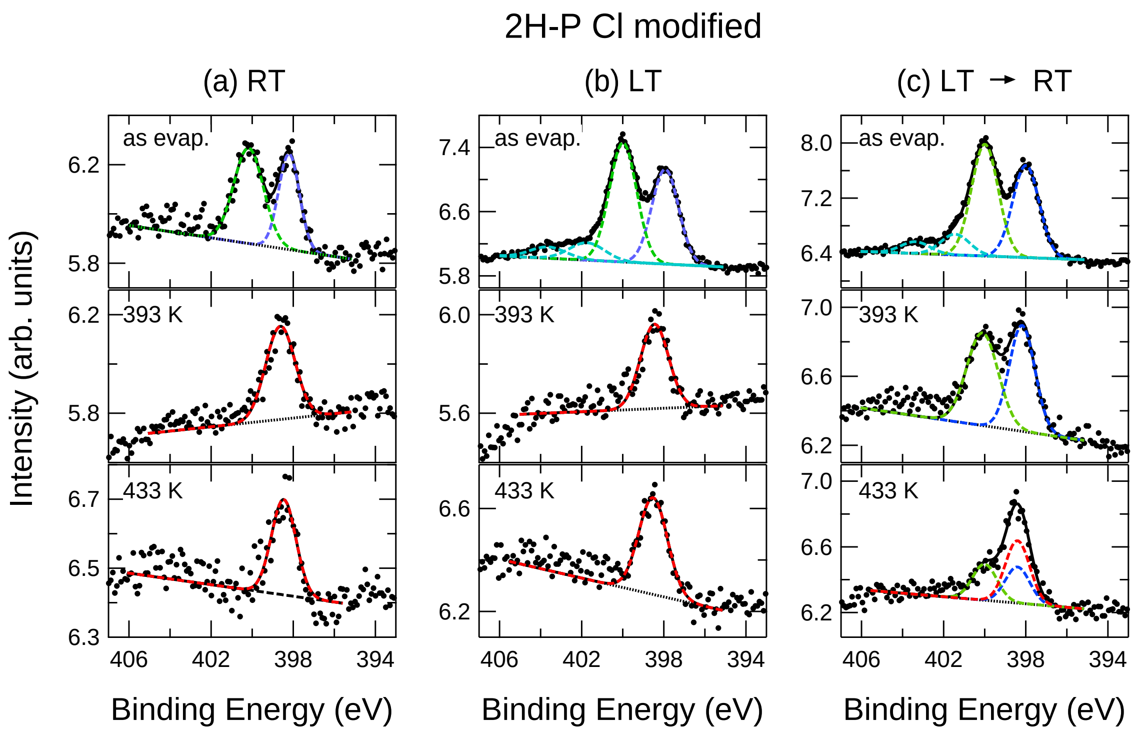


FIG. S**7** Influence of the molecular orientation of 2H-P/Cu(111) on the self-metalation. The data correspond to chlorine contaminated films, as the pure films were less stable. (a) Bilayer grown at room temperature: all molecules (flat orientation) are metalated at 393 K, as indicated by the transition from a two-peak structure (NH and =N) to a single peak (NCu) in the N1s signal. (b) The same could be observed for (flat) multilayers grown at low temperatures. (c) In contrast, the multilayer grown at low temperatures and warmed up slowly to room temperature, i.e., maintaining the molecules in the perpendicular orientation (Fig. S6), only partially metalates at elevated temperatures (433 K).

## REFERENCES

[1]Christian Mück-Lichtenfeld and Stefan Grimme. Structure and binding energies of the porphine dimer. Molecular Physics: An International Journal at the Interface Between Chemistry and Physics, 105:2793–2798, 2007.
